# Supplementary material for: GenSpan: Generation-Calibrated Motion Span Priors for Multi-Verb Video Corpus Moment Retrieval
Source: arXiv:2603.22121 source file (2026-06-03)
Supplement: Supplementary file 1 [file paper_appendix.tex]

% =========================================================================
% FIGURE 1: TOP OF PAGE 1 (Using strip environment)
% =========================================================================
% --- Figure 1: Pipeline ---
\begin{figure}[t!]
    \centering
    \includegraphics[width=1.0\linewidth]{figures/fig_a1_pipeline.png} 
    \caption{Overview of the video clipping pipeline. The upper section displays the main preview window showing a dyadic dance interaction scene. The lower section illustrates the timeline track with keyframes of the clipped sub-video.}
    \label{fig:capcut_pipeline}
\end{figure}

% --- Figure 2: File Structure ---
% Placed here to float to the top of the next column or page naturally
\begin{figure}[t!]
    \centering
    \includegraphics[width=0.9\linewidth]{figures/fig_a2_structure.png}
    \caption{Hierarchical file structure of the DuaLMHR dataset. The organization separates video and text modalities under a common root, further categorized by interaction type to support scalable data loading.}
    \label{fig:dataset_structure}
\end{figure}

% =========================================================================
% FIGURES 2 & 3: TOP OF PAGE 2
% =========================================================================
% 在第1页的代码中声明 figure*，LaTeX 会自动将其浮动到第2页顶端
\begin{figure*}[t!]
    \centering
    \includegraphics[width=0.98\textwidth]{figures/幻灯片1.PNG}
    \caption{Category distribution of the DuaLMHR training data. The plot illustrates the percentage of top action verbs, exhibiting a characteristic long-tail distribution. High-frequency interactions (e.g., \textit{stand}, \textit{hold}) are abundant, while our data engine strategy ensures sufficient coverage for complex, lower-frequency actions (e.g., \textit{manipulate}, \textit{sway}) to promote robust generalization.}
    \label{fig:long_tail_distribution}
\end{figure*}

% =========================================================================
% INTRODUCTION
% =========================================================================
\noindent This supplementary material provides comprehensive details regarding the data engine, construction pipeline, annotation process, and downstream applications of the DuaLMHR dataset. The document is organized as follows: 

\textbf{Section~\ref{sec:Long-tail Distribution Analysis}} introduces the long-tail distribution analysis. 

\textbf{Section~\ref{sec:construction}} details the video clipping pipeline and dataset organization.

\textbf{Section~\ref{sec:annotation}} describes the annotation methodology using Gemini 3.0 Pro. 

Finally, \textbf{Section~\ref{sec:downstream_tasks}} elaborates on the four downstream tasks and benchmarks.

% =========================================================================
% SECTION A: DATA ENGINE
% =========================================================================
\section{Long-tail Distribution Analysis}
\label{sec:Long-tail Distribution Analysis}
As illustrated in Figure~\ref{fig:long_tail_distribution}, real-world human interactions exhibit an inherent long-tail distribution. While common atomic actions such as ``stand'' or ``step'' dominate the frequency spectrum, complex interactions like ``manipulate'' or ``synchronize'' appear far less frequently. Despite their scarcity, these long-tail instances are indispensable for achieving a high-level, nuanced understanding of human dynamics, as they often contain the most significant semantic information.

To mitigate the bias stemming from this inherent imbalance, we implement a sampling strategy inspired by curriculum learning. By leveraging fine-grained action category labels, we maintain continuous monitoring of the interaction distribution throughout the data engine's workflow. This facilitates dynamic adjustments to data sourcing, allowing us to proactively prioritize samples from the long tail of the distribution and rectify skewness before proceeding to the annotation phase.

Specifically, our collection protocol progresses from simple interactions to increasingly intricate dynamics. We place particular emphasis on structurally complex actions (e.g., \textit{reach}, \textit{pull}) and highly continuous interactions (e.g., \textit{sway}, \textit{twist}) that typically reside in the long tail. This approach prevents the dataset from being overwhelmed by trivial behaviors, thereby providing a comprehensive and balanced training ground that enhances the robustness of motion understanding models in open-world scenarios.

% =========================================================================
% SECTION B: DATASET CONSTRUCTION
% =========================================================================
\section{Dataset Construction Pipeline}
\label{sec:construction}

\subsection{Video Clipping Pipeline}
Following the data sourcing phase described in Section~\ref{sec:annotation}, the video processing pipeline utilizes \textit{CapCut}, a professional editing tool shown in Figure~\ref{fig:capcut_pipeline}. This platform supports precise frame-level trimming and multi-track editing, which facilitates the handling of long video sequences. 

The clipping procedure is as follows:
In the subsequent filtering and export phase, we enforce rigorous quality control protocols to ensure high data fidelity. We prioritize video segments with low background complexity, high resolution, and an absolute absence of scene transitions. To maintain visual integrity, the torsos of both participants must remain clearly visible and free from significant occlusion or environmental interference throughout the entire action cycle; segments with severe visual obstructions are systematically pruned. Finally, to preserve rich motion dynamics while maintaining consistency for model training, all selected subsequences are standardized to a duration ranging from $5$ to $15$ seconds and exported as standalone video files.

In the subsequent filtering and export phase, we enforce rigorous quality control protocols to ensure high data fidelity. We prioritize video segments with low background complexity, high resolution, and an absolute absence of scene transitions. To maintain visual integrity, the torsos of both participants must remain clearly visible and free from significant occlusion or environmental interference throughout the entire action cycle; segments with severe visual obstructions are systematically pruned. Finally, to preserve rich motion dynamics while maintaining consistency for model training, all selected subsequences are standardized to a duration ranging from $5$ to $15$ seconds and exported as standalone video files.

\subsection{Dataset Organization and Structure}
The resulting dataset is organized into a hierarchical structure to ensure efficient management and accessibility, as depicted in Figure~\ref{fig:dataset_structure}. 

The root directory, named ``DuaLMHR,'' contains two primary sub-directories: ``Video'' and ``Text.'' These files are further stratified by interaction category (e.g., Daily Social, Dance, Medical Care, Sports). Additionally, we store the classification labels (contact vs. non-contact) and difficulty scores for each video in separate JSON files using a key-value pair format.

% =========================================================================
% SECTION C: ANNOTATION
% =========================================================================
\section{Dataset Annotation}
\label{sec:annotation}

\begin{figure*}[t!]
    \centering
    \includegraphics[width=0.98\textwidth]{figures/figure3.png}
    \caption{The full annotation prompt used for Gemini 3.0 Pro. The prompt incorporates strict constraints: 1) Targeting dyadic human motion sequences. 2) Requiring strictly gender-neutral descriptions. 3) Prohibiting high-level semantic labels. 4) Mandating fine-grained spatiotemporal joint details.}
    \label{fig:gemini_prompt_example}
\end{figure*}

This paper employs large-scale invocations of Gemini 3.0 Pro to annotate videos along the motion dimension. The annotation prompt design is critical to ensuring high-quality, physically grounded descriptions.

As shown in Figure~\ref{fig:gemini_prompt_example}, to ensure the extraction of precise kinematic features from videos rather than high-level semantics, the prompt incorporates strict constraints. It mandates descriptions that emphasize fine-grained spatiotemporal joint details of upper and lower limbs as well as torso orientations, explicitly prohibiting high-level semantic labels (e.g., ``dancing'') to focus on the physical processes of actions.

\subsection{Contact and Non-Contact Classification}
To ensure the precise categorization of contact and non-contact interactions, we implemented a multi-stage inference pipeline. Specifically, we first wait for the generation of fine-grained motion descriptions from the preceding step, and subsequently utilize a Large Language Model to infer the corresponding classification labels based on these textual descriptions. This decoupling strategy effectively mitigates the "hallucination" phenomenon commonly observed in concurrent multi-task generation, ensuring high logical consistency between the semantic descriptions and the final categorical judgments. Finally, the classification results are persistently stored in a JSON metadata file as key-value pairs, with the unique video identifier (ID) as the key and the corresponding category as the value.

\subsection{Difficulty Classification}
Difficulty classification is similar to contact and non-contact categorization. The five indicators for difficulty levels are: 1) Simple upper body actions; 2) Simple upper body actions + movement; 3) Compound upper body actions; 4) Compound actions + movement; 5) Natural scene behaviors.

% =========================================================================
% SECTION D: DOWNSTREAM TASKS
% =========================================================================
\section{Downstream Tasks}
\label{sec:downstream_tasks}

Our dataset provides rich annotations for dual-person interactions, enabling four distinct downstream tasks. These tasks range from temporal localization in the video domain to temporal grounding in the 3D motion domain. In this section,we provide a detailed elaboration on the transfer principles and experimental results for each respective task.

% -------------------------------------------------------------------------
% Task 1: Video TAL
% -------------------------------------------------------------------------
\subsection{Temporal Video Grounding}
\label{subsec:video_tal}
Our dataset supports Video Temporal Action Localization (TAL) in a text-conditioned setting, enabling models to localize specific interaction events within untrimmed video sequences based on textual queries.

\paragraph{Data Construction \& Ground Truth.}
Leveraging its construction via the extraction of specific events from extended raw sequences, our dataset inherently retains precise ground-truth start and end timestamps from the manual editing phase. To enhance scalability, these temporal boundaries can also be automatically recovered through image similarity matching (e.g., $SSIM > 0.8$) between the clipped segments and the source frames. In conjunction with our fine-grained textual annotations, this framework seamlessly facilitates the \textit{Text-Conditioned TAL} task: models are tasked with predicting the temporal boundaries (start and end indices) within the original video for a given natural language query.

\paragraph{Benchmarks.}
We benchmark several state-of-the-art methods using a standard split (70\% train, 15\% validation, 15\% test) and report the Mean Average Precision (mAP) at specific IoU thresholds. As shown in Table~\ref{tab:video_tal}, AdaTAD achieves the highest performance, demonstrating the dataset's challenge and utility.

\begin{table}[t!]
    \centering
    \caption{Benchmark results for Temporal Video Grounding on our dataset.}
    \label{tab:video_tal}
    \begin{tabular}{l c c c}
        \toprule
        Method & Year & R@0.5 & R@0.7 \\
        \midrule
        G-TAD~\citep{xu2020gtad}          & 2020 & 32.1 & 18.4 \\
        TemporalMaxer~\citep{benchmark2023} & 2023 & 38.7 & 24.2 \\
        AdaTAD~\citep{liu2023adatad}      & 2024 & 42.5 & 27.6 \\
        PLOT-TAL~\citep{fish2025plottal} & 2025 & 45.3 & 29.8 \\
        QROT~\citep{liu2025qrot}          & 2025 & 47.9 & 31.5 \\
        \bottomrule
    \end{tabular}
\end{table}

% -------------------------------------------------------------------------
% Task 2: Motion Grounding
% -------------------------------------------------------------------------
\subsection{Temporal Motion Grounding}
\label{subsec:motion_grounding}
This task extends temporal localization into the domain of 3D motion, focusing on grounding textual queries to temporal segments within 3D human interaction sequences.

\paragraph{From Video to Motion.}
Once the temporal boundaries are established in the video domain (as detailed in Section~\ref{subsec:video_tal}), they exhibit a direct one-to-one correspondence with the timestamps in the motion domain. This temporal synchronization facilitates the \textit{Interaction Motion Temporal Grounding} task, which requires the model to localize specific motion segments within a continuous 3D sequence based on textual queries. By leveraging the source videos and employing robust 3D motion reconstruction frameworks (e.g., VIBE or ROMP), researchers can derive comprehensive 3D interaction sequences to perform high-fidelity temporal grounding evaluations.

\paragraph{Benchmarks.}
We evaluate baselines on our test set, reporting Recall@IoU (R@0.5 and R@0.7) to measure precise localization capabilities. As presented in Table~\ref{tab:motion_grounding}, ZOMG demonstrates superior performance in capturing complex interaction dynamics.

\begin{table}[t!]
    \centering
    \caption{Performance comparison on the Temporal Motion Grounding task.}
    \label{tab:motion_grounding}
    \begin{tabular}{l c c c}
        \toprule
        Method & Year & R@0.5 & R@0.7 \\
        \midrule
        TMN~\citep{tmn2020}            & 2020 & 25.6 & 12.3 \\
        SeViLA~\citep{sevila2023}      & 2023 & 31.4 & 17.8 \\
        TM-Mamba~\citep{tmmamba2024}   & 2024 & 35.2 & 20.5 \\
        MLP~\citep{mlp2024}            & 2024 & 37.1 & 22.4 \\
        ZOMG~\citep{zomg2025}          & 2025 & 39.8 & 24.7 \\
        \bottomrule
    \end{tabular}
\end{table}

\subsection{Video Interaction Action Localization}
\label{subsec:video_action_loc}
This task addresses the spatial-temporal localization of actions within video clips, specifically focusing on human-object and human-human motion interactions (e.g., ``carry'' or ``watch'').

\paragraph{Setup and Metrics.}
Leveraging InterX-style annotations, which combine \textbf{spatial bounding boxes} with temporal action spans, we provide high-quality ground truth for end-to-end localization. Baselines are evaluated on motion-augmented videos. We report mAP@0.5 and Accuracy in Table~\ref{tab:video_action_loc}, where LAIN achieves state-of-the-art results.

\paragraph{Benchmarks.}
As illustrated in Table~\ref{tab:video_action_loc}, performance has improved steadily from early graph-based methods to recent transformer architectures. Notably, \textbf{LAIN} (2025) sets the state-of-the-art in zero-shot scenarios with 40.3\% mAP@0.5 and 49.2\% Accuracy, demonstrating its superior capability in modeling the intricate spatio-temporal dynamics of dual-person interactions via context prompting.

\begin{table}[t!]
    \centering
    \caption{Performance comparison on Video Spatio-Temporal Action Localization.}
    \label{tab:video_action_loc}
    \begin{tabular}{l c c c}
        \toprule
        Method & Year & mAP@0.5 & Acc \\
        \midrule
        IP-Net~\citep{ipnet2020} & 2020 & 28.4 & 35.7 \\
        SCOPE~\citep{scope2023}  & 2023 & 34.2 & 42.1 \\
        HORP~\citep{horp2025}    & 2025 & 37.8 & 46.5 \\
        LAIN~\citep{lain2025}    & 2025 & 40.3 & 49.2 \\
        \bottomrule
    \end{tabular}
\end{table}

% -------------------------------------------------------------------------
% Task 4: 3D Interaction
% -------------------------------------------------------------------------
\subsection{3D Human Interaction Action Localization}
\label{subsec:3d_hoi_loc}
Finally, we propose the task of \textbf{3D Human Interaction Localization}. By leveraging our exhaustive 3D HOI annotations, this task focuses on localizing specific interaction segments directly within reconstructed motion meshes, thereby effectively resolving the depth and occlusion ambiguities inherent in 2D video spaces.

\paragraph{Benchmarks.}
This task is of paramount importance for robotics and character animation, where precise physical contact understanding is required. We evaluate several baselines adapted from prominent recent studies, reporting mAP@0.5 and Accuracy. As demonstrated in Table~\ref{tab:3d_hoi_localization}, \textbf{Human-X} (2025) currently leads the benchmark. Its superior performance underscores the critical role of modeling fine-grained physical constraints and contact dynamics in 3D space compared to earlier transformer-based or control-centric approaches.

\begin{table}[t!]
    \centering
    \caption{Performance of baselines on 3D Human Interaction Action Localization (sorted by performance).}
    \label{tab:3d_hoi_localization}
    \begin{tabular}{l c c c}
        \toprule
        Method & Year & mAP@0.5 & Acc \\
        \midrule
        InterFormer~\citep{chopin2023interactiontransformerhumanreaction} & 2023 & 22.5 & 28.3 \\
        InterControl~\citep{intercontrol2024}  & 2024 & 27.4 & 33.6 \\
        InterMask~\citep{javed2024intermask} & 2024 & 30.1 & 36.8 \\
        Intergen~\citep{interact2025} & 2024 & 33.7 & 40.2 \\
        Human-X~\citep{ji2025towards} & 2025 & 36.5 & 43.9\\
        \bottomrule
    \end{tabular}
\end{table}
% =========================================================================
% SECTION E: ADDITIONAL VISUALIZATIONS
% =========================================================================
\section{Additional Visualizations}
\label{sec:more_viz}

We provide additional qualitative examples of our dataset in Figure~\ref{fig:more_viz} (see next page). These visualizations comprehensively demonstrate the richness and high fidelity of our data engine. 

As illustrated in the following figure, we present a diverse set of samples covering various interaction types. Each sample includes the raw video motion sequence, the corresponding 3D motion mapping (reconstructed mesh), and the fine-grained textual prompt. This alignment highlights the dataset's capability to capture intricate physical dynamics and semantic details, supporting the complex downstream tasks discussed in Section~\ref{sec:downstream_tasks}.

% Force the figure to the next page
\clearpage

% =========================================================================
% FIGURE: VISUALIZATION GALLERY
% =========================================================================
\begin{figure*}[t!]
    \centering
    % Replace with your actual large visualization image file
    \includegraphics[width=1.0\textwidth]{figures/fig_visualization_gallery.png}
    \caption{Extended qualitative examples from the DuaLMHR dataset. This figure showcases a selection of video clips alongside their processed annotations. \textbf{Top Row:} Sample frames from the original video clips capturing diverse dyadic interactions. \textbf{Middle Row:} The corresponding 3D motion reconstruction visualized as SMPL meshes, demonstrating precise spatial alignment. \textbf{Bottom Row:} The associated fine-grained text prompts that describe the temporal evolution of the interaction. These examples verify the robustness of our pipeline in handling complex occlusions and multi-person dynamics.}
    \label{fig:more_viz}
\end{figure*}
% ... 前面是你的正文内容 ...

% Ensure references start on a new page after the large figure
\clearpage
